# Supplementary material for: A Simple Electrostatic Model for the Hard-Sphere Solute Component of Nonpolar Solvation
Source: arXiv:2005.13019 source file (2020-03-13)
Supplement: Supplementary file 2 [file suppmethods.tex]

\begin{figure}[!h]
\centering
\includegraphics[width=0.3\textwidth]{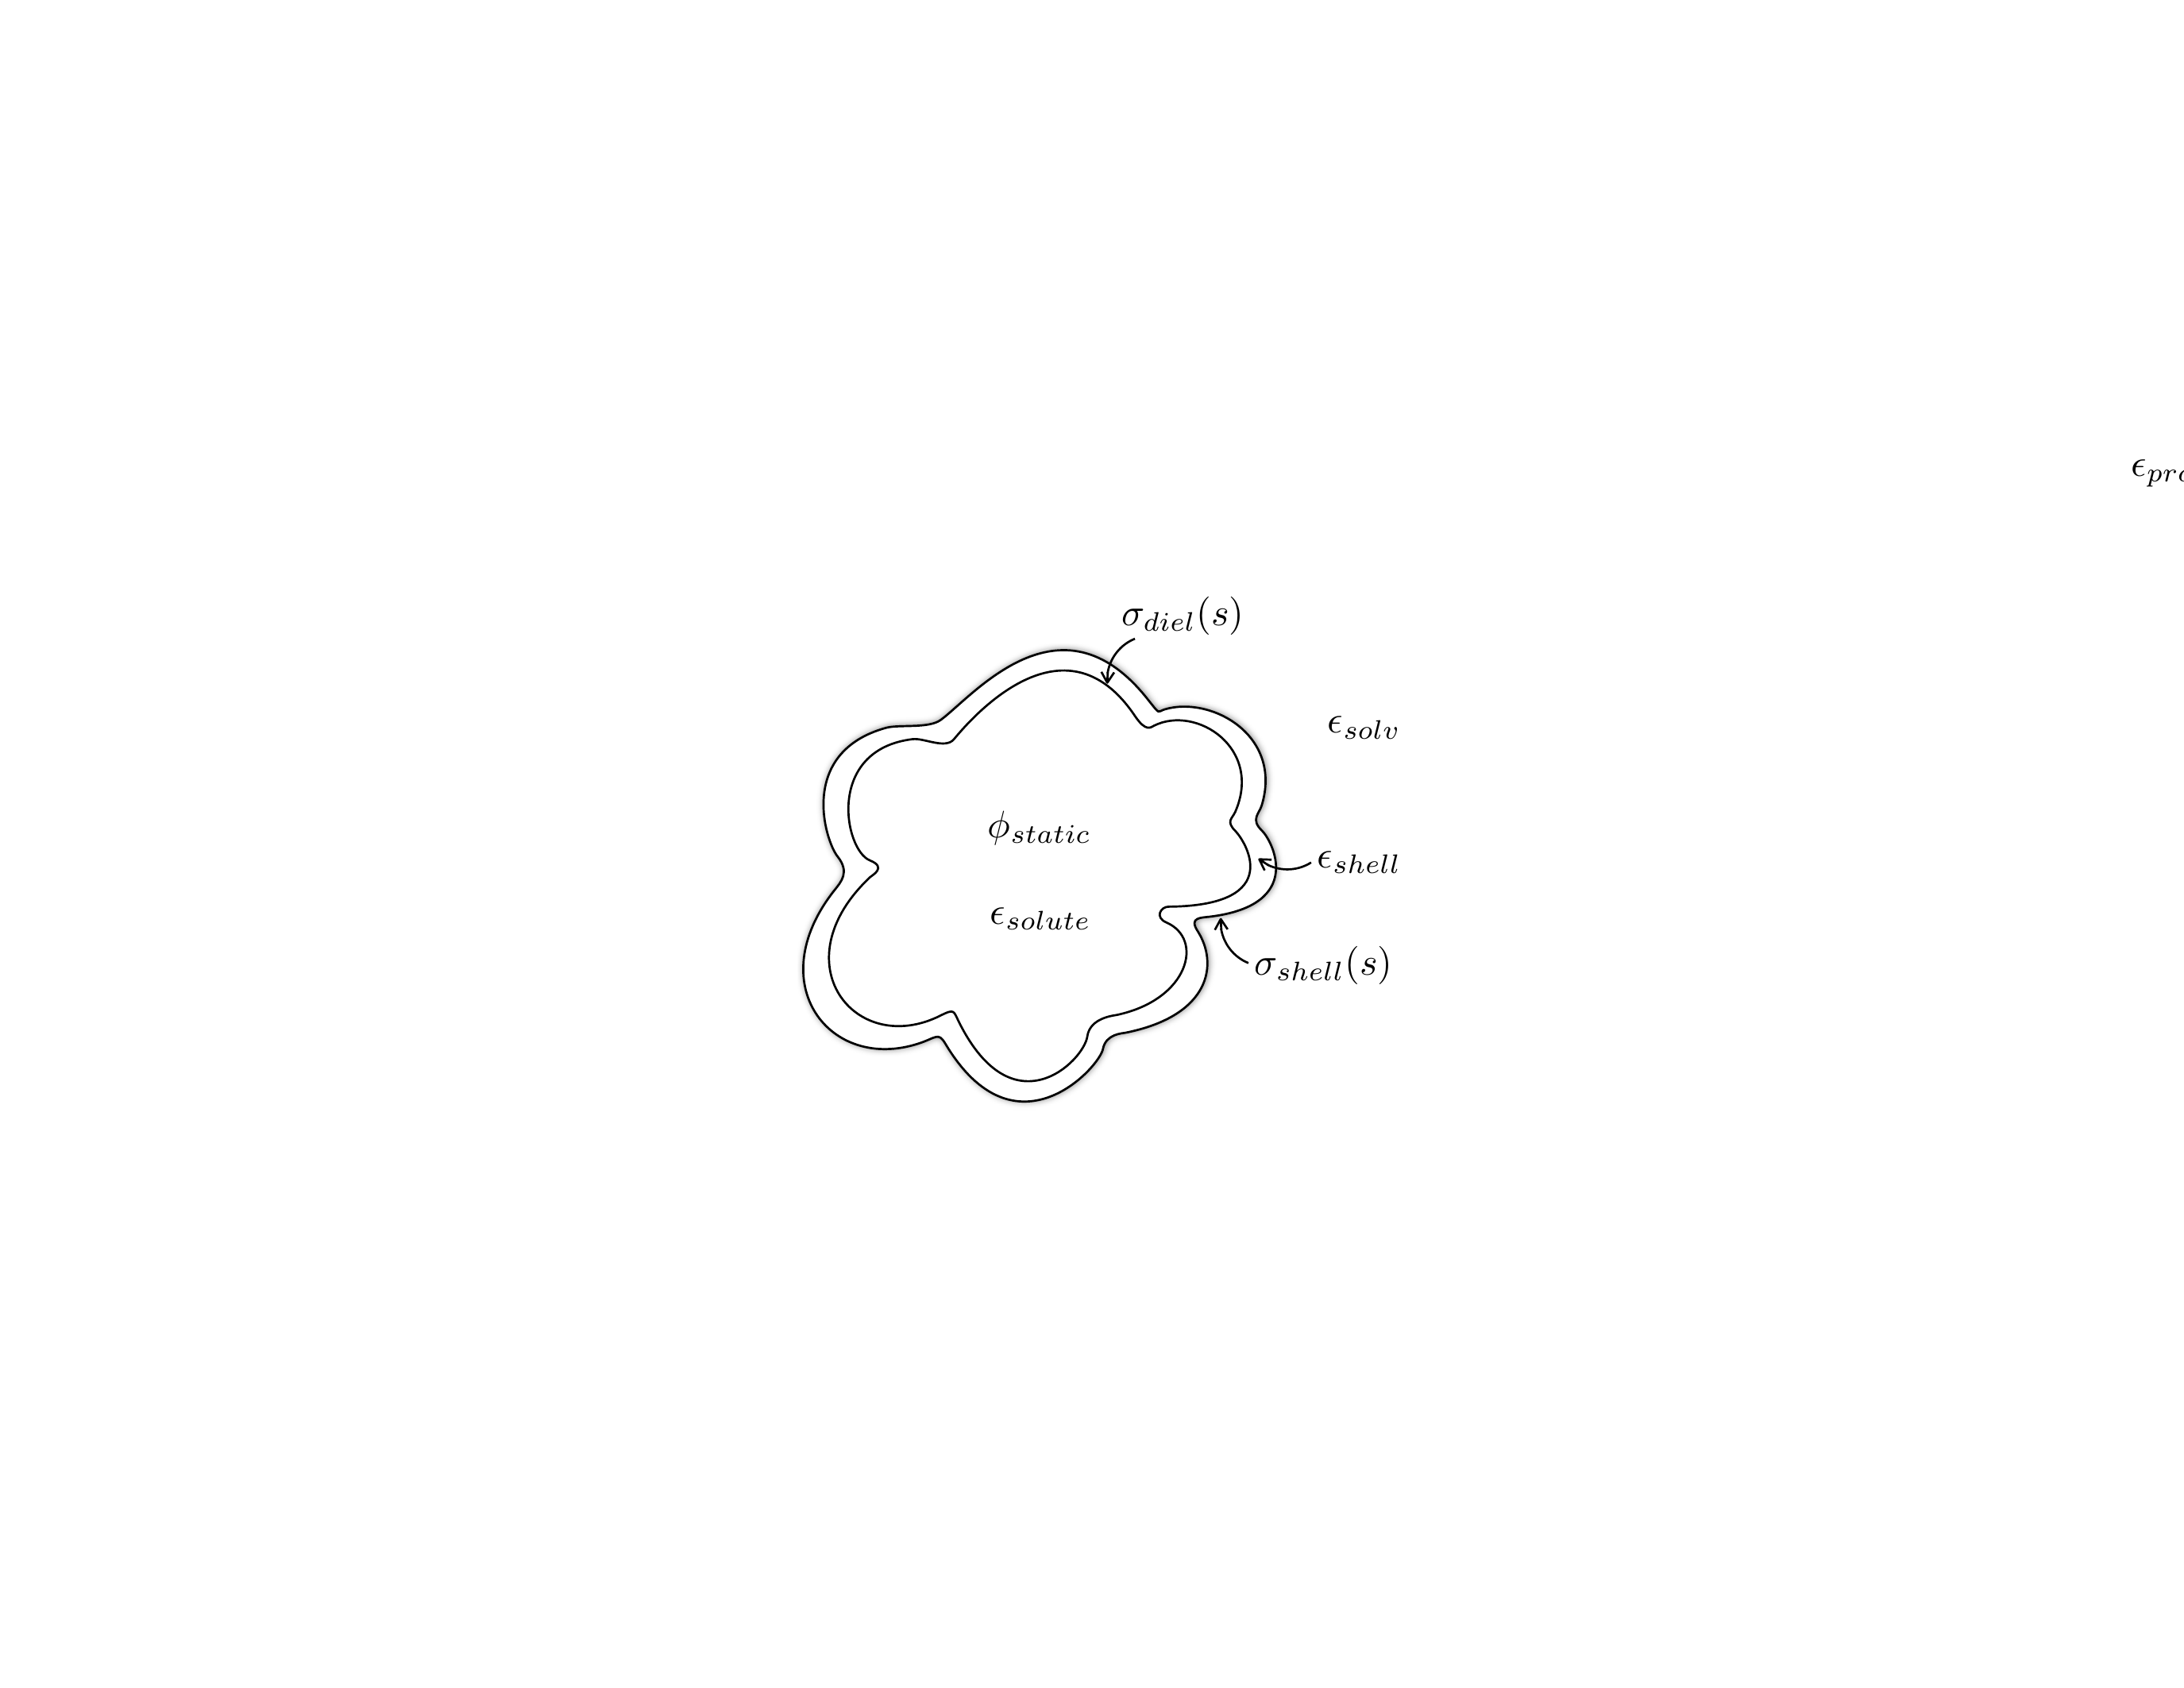}
\caption{Capacitor model of a solute.}
\label{fig:capacitor}
\end{figure}

Figure \ref{fig:capacitor} is a representation of an uncharged solute immersed in a solvent, with a Stern layer between them.
The interface between the solute and Stern layer is called the solvent-excluded surface (SES), whereas the solvent-accessible surface (SAS) is one water radius away ($\sim 1.4$\AA), in the limit between the Stern layer and the solvent. 
In this model, we place surface charge densities at the SES ($\sigma_{\text{SES}}$) and SAS ($\sigma_{\text{SAS}}$) to reproduce the electrostatic potential distribution seen in an uncharged solute, and compute the energy from this setup.

The electrostatic potential in the Stern layer is induced by the surface charge distributions as follows

In this case, as the electrostatic potential is constant in the solute and solvent, there is no need to consider the apparent surface charge from the jump in dielectric constant (see Supplementary Material).

We know the potential just inside the SES is $\phi_\text{static}$, whereas the potential just outside the SAS must be zero.
Then, considering that the potential is continuous across dielectric interfaces and surface charges, we can evaluate Equation \eqref{eq:surface_charge} on the SES and SAS, to get
%
%\begin{align}\label{eq:surface_charge_eval}
%\phi(\mathbf{r}_\text{SES}) = \phi_\text{static} &= \oint_\text{SES} \frac{\sigma_\text{SES}(\mathbf{r}')}{4\pi \epsilon_\text{Stern}|\mathbf{r}_\text{SES}- \mathbf{r}'|} \text{d}\mathbf{r}' + \oint_\text{SAS} \frac{\sigma_\text{SAS}(\mathbf{r}')}{4\pi \epsilon_\text{Stern}|\mathbf{r}_\text{SES}- \mathbf{r}'|} \text{d}\mathbf{r}' \nonumber \\
%\phi(\mathbf{r}_\text{SAS}) = 0 &= \oint_\text{SES} \frac{\sigma_\text{SES}(\mathbf{r}')}{4\pi \epsilon_\text{Stern}|\mathbf{r}_\text{SAS}- \mathbf{r}'|} \text{d}\mathbf{r}' + \oint_\text{SAS} \frac{\sigma_\text{SAS}(\mathbf{r}')}{4\pi \epsilon_\text{Stern}|\mathbf{r}_\text{SAS}- \mathbf{r}'|} \text{d}\mathbf{r}',
%\end{align}
%
%which can be written in matrix form as
%
\begin{equation}\label{eq:matrix}
\left[
\begin{array}{c c}
V_\text{SES} & V_\text{SES}\\
V_\text{SAS} & V_\text{SAS}
\end{array}
\right]
\left[
\begin{array}{c}
\sigma_\text{SES}\\
\sigma_\text{SAS}
\end{array}
\right]
=
\epsilon_\text{Stern}\left[
\begin{array}{c}
\phi_\text{static}\\
0 
\end{array}
\right]
\end{equation}
Here, $V_{\Gamma_1}(\psi_{\Gamma_2}) = \oint_{\Gamma_2} \frac{\psi(\mathbf{r}')}{4\pi|\mathbf{r}_{\Gamma_1} - \mathbf{r}'|}\text{d}\mathbf{r}'$ is the single-layer potential of the distribution $\psi$ on $\Gamma_2$, evaluated on a point located in $\Gamma_1$.
%
%\begin{equation}\label{eq:single_layer}
%V_{\Gamma_1}(\psi_{\Gamma_2}) = \oint_{\Gamma_2} \frac{\psi(\mathbf{r}')}{4\pi|\mathbf{r}_{\Gamma_1} - \mathbf{r}'|}\text{d}\mathbf{r}'.
%\end{equation}

We solve for $\sigma_\text{SES}$ and $\sigma_\text{SAS}$ in Equation \eqref{eq:matrix} with a boundary element method (BEM) using the \texttt{bempp} library \cite{SmigajETal2015}.
The BEM generates a numerical version of Equation \eqref{eq:matrix} starting from a surface discretized in flat triangular panels (obtained using \texttt{msms} \cite{SannerOlsonSpehner1995}), and solves for $\sigma_\text{SES}$ and $\sigma_\text{SAS}$. 
With \texttt{bempp}, we assume a piecewise constant distribution of $\sigma_\text{SAS}$ and $\sigma_\text{SES}$ on the molecular surface, and use a Galerkin approach to generate a matrix which we solve with a GMRES algorithm.

Having the surface charge distributions, and considering that the potential on the SAS is zero, we can compute the energy with 
\begin{equation}\label{eq:energy}
\Delta G_\text{cav} = \oint_\text{SES} \phi_\text{static}\sigma_\text{SES}(\mathbf{r})\text{d}\mathbf{r}
\end{equation}

By using continuum electrostatic theory, the solvent degrees of freedom are averaged out, making Equation \eqref{eq:energy} a free energy calculation \cite{RouxSimonson1999}.
In particular, $\Delta G_\text{cav}$ is the electrostatic contribution to the difference in Gibbs free energy between the solvent in bulk state (no free energy) and with a cavity, which equals the reversible work required to generate the void where the solute will fit. 
%This should not be confused with the so-called solvent reorganization energy \cite{YuKarplus1988,Lazaridis2000,GallicchioKuboLevy2000}, which refers to the binding energy of a single solvent molecule as it is surrounded by the rest of the solvent.
%That solvent reorganization energy contributes to the internal energy, and not the free energy directly.

%%%%%\subsection{A surface integral approach for $\Delta G_\text{vdw}$}
Levy {\it et al.} \cite{LevyZhangGallicchioFelts2003} used a continuum description to compute the energy from solute-solvent dispersion interactions based on the integral of the Lennard-Jones potential over the solvent. Later, Bardhan {\it et al.}\cite{BardhanETal2005} used the divergence theorem to reformulate it as
\begin{equation}\label{eq:vdw_energy}
\Delta G_\text{disp} = \sum_i \oint_\text{SAS} \rho_w \frac{\partial}{\partial \mathbf{n}}\left( \frac{A_i}{90|\mathbf{r} - \mathbf{r}_i|^{10}}
- \frac{B_i}{12|\mathbf{r} - \mathbf{r}_i|^4}\right) \text{d}\mathbf{r}  
\end{equation}
%
%\begin{equation}\label{eq:vdw_volume}
%\Delta G_\text{vdw} = \sum_i \int_\text{solvent} \rho_w \left(\frac{A_i}{|\mathbf{r}-\mathbf{r}_i|^{12}} - \frac{B_i}{|\mathbf{r}-\mathbf{r}_i|^{6}}\right) \text{d}\mathbf{r}
%\end{equation}
%
where $\rho_w$ is the solvent number density, $A_i$ and $B_i$ are the Lennard-Jones parameters for atom $i$, and the sum is over the solute's atoms. Also, the unit vector $\mathbf{n}$ points away from the SAS. 
%In the work by Bardhan {\it et al.} \cite{BardhanETal2005}, the authors use the divergence theorem to represent Equation \eqref{eq:vdw_volume} as a surface integral, which gives
%
%
%where $\mathbf{n}$ is a unit vector normal to the SAS, pointing into the solvent.
The formulation in Equation \eqref{eq:vdw_energy} is very convenient to our model, as it only requires a mesh over the SAS, which we already have from the calculation of $\Delta G_\text{cav}$.

It is well known that the water density increases near interfaces CITE. 
We account for this fact by considering a thin layer that is one water molecule radius thick ($1.4$\AA) beyond the SAS with a higher density, in our case, set to $1.8\rho_w$.
This, however, can be seen as a fitting parameter for the dispersion energy.

%-------------------
%The nonpolar component of the solvation energy is usually decomposed into $\Delta G_\text{cav} + \Delta G_\text{disp}$, the sum of the energy required to generate the cavity plus the energy from the solute-solvent dispersion interaction, respectively.\cite{GallicchioZhangLevy2002} This decomposition is discussed in the Supplementary Material and sketched in Figure S1. Here, we detail the models used for $\Delta G_\text{cav}$ and $\Delta G_\text{disp}$. 
